# Supplementary material for: Long-range translational order and hyperuniformity in two-dimensional chiral active crystal
Source: arXiv:2402.19192 source file (2025-03-02)
Supplement: Supplementary file 1 [file supplement.pdf]

# Supplementary material for "Long-range translational order and hyperuniformity in two-dimensional chiral active crystal"

Yuta Kuroda, Takeshi Kawasaki, and Kunimasa Miyazaki
*Department of Physics, Nagoya University, Nagoya 464-8602, Japan*

## S1. SETUP OF NUMERICAL SIMULATION

We performed the numerical simulation for Eqs. (1) and (2) in the main text. The system size is given by $L_x \times L_y$, and the periodic boundary condition is imposed. We used the harmonic potential for the pairwise interaction:

$$U(r) = \frac{\epsilon}{2}\left(1 - \frac{r}{\sigma}\right)^2 \theta(\sigma - r), \tag{S1}$$

where $\sigma$ is the diameter of a particle and $\theta(\cdot)$ is the Heaviside step function. We chose $\sigma$ and $\tau = \sigma/v_0$ as the units of length and time scales. The control parameters in this system are dimensionless orbital radius $R/\sigma = 1/(\Omega\tau)$, rotational diffusion constant $D\tau$, energy ratio $\epsilon/(v_0\zeta\sigma)$, and the packing fraction $\varphi = \pi\sigma^2 N/(4L_xL_y)$. We fixed the energy ratio as $\epsilon/(v_0\zeta\sigma) = 40$. The initial value of the angle of the orientation, $\phi_j(0)$, is given by the uniform distribution on $[0, 2\pi)$. We integrated the equations of motion by the Euler method with a time step $\Delta t = 10^{-3}\tau$. The ratio of the system size is given by $L_x : L_y = 7 : 4\sqrt{3}$ to accommodate the hexagonal structure. Using the lattice constant $\ell_0$, the packing fraction is written as $\varphi = \pi\sigma^2/(2\sqrt{3}\ell_0^2)$. We studied only the region $\ell_0 \leq \sigma$ to avoid the absorbing phase transition.

## S2. GLOBAL TRANSLATIONAL ORDER PARAMETER

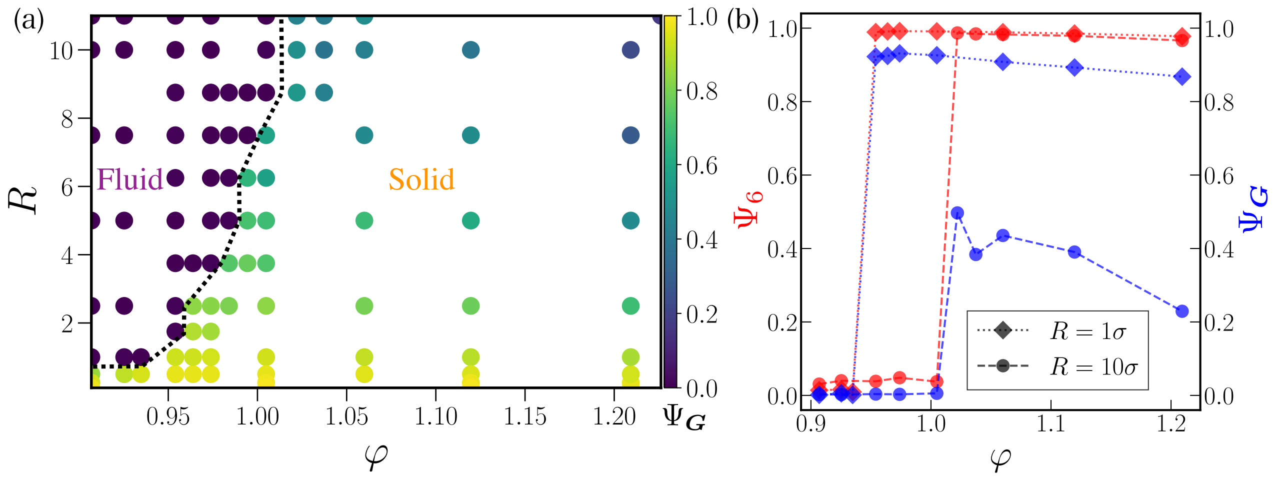


FIG. S1. (a) The phase diagram in the $(\varphi, R)$ plane at $N = 12600$. The color represents the global translational order parameter $\Psi_G$. (b) The global hexatic (red color) and translational (blue color) order parameter as a function of the packing fraction $\varphi$. The diamond symbols (♦) and filled circles (•) are the data at $R = 1\sigma$ and $10\sigma$, respectively.

In Fig. S1(a), we show the phase diagram in the $(\varphi, R)$ plane colored by the global translational order parameter $\Psi_G = |\sum_{j=1}^{N} \langle \rho_G(\boldsymbol{r}_j)\rangle|/N$. Comparing with Fig. 1 in the main text, one observes that the phase boundary between fluid and solid phases determined by $\Psi_6$ is identical to that determined by $\Psi_G$. Figure S1(b) depicts the global hexatic and translational order, $\Psi_6$ and $\Psi_G$, as a function of the packing fraction $\varphi$, at $R = 1\sigma$ and $10\sigma$. For both $R$'s, $\Psi_6$ and $\Psi_G$ jump to the finite values at the same $\varphi$. This suggests the absence of the hexatic phase and that the transition is discontinuous. However, the system size of the current simulation is not large enough to conclusively determine the nature of the transition. We leave a more careful study of the behavior near the phase boundary to future work.

## S3. DENSITY DEPENDENCE OF THE CORRELATION FUNCTIONS

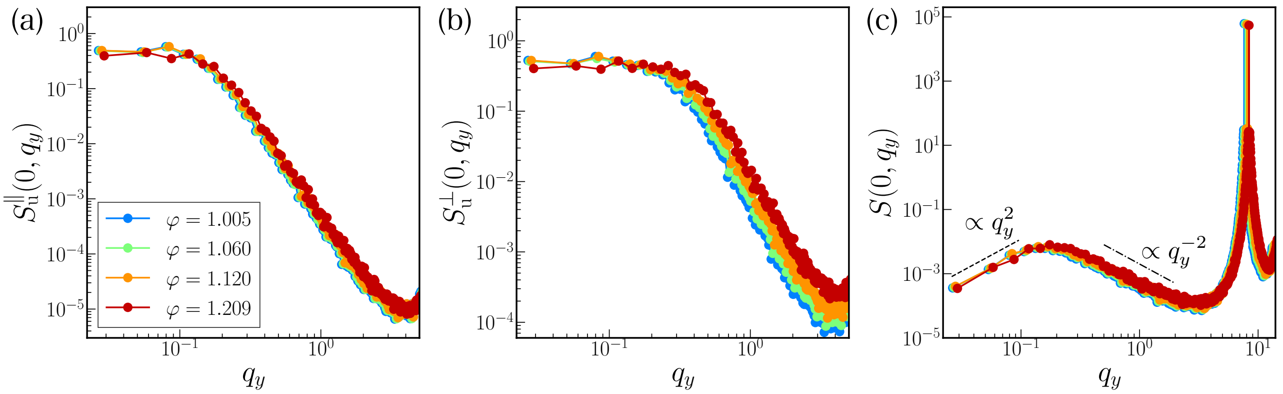


FIG. S2. The density dependence of the correlation functions in the Fourier space at $R = 1\sigma$, $D = 0$, and $N = 72576$. Panel (a) and (b) are the longitudinal and transverse displacement correlations, respectively. The static structure factor is shown in panel (c).

Figure S2 shows the correlation functions for several packing fractions. The qualitative behavior of all correlation functions is unaltered by $\varphi$.

## S4. TRANSLATIONAL ORDER IN LINEAR ELASTIC THEORY

Here we calculate the correlation function of the translational order parameter from the linear elastic theory. In the coarse-grained field description, the translational order parameter is written as $\rho_{\boldsymbol{G}}(\boldsymbol{r}) = e^{i\boldsymbol{G}\cdot\boldsymbol{u}(\boldsymbol{r})/\rho}$, where $\rho$ is the mean density. The correlation function is defined by

$$C_{\boldsymbol{G}}(r) = \langle \rho_{\boldsymbol{G}}(\boldsymbol{r})\rho^*_{\boldsymbol{G}}(\boldsymbol{0})\rangle = \left\langle e^{i\boldsymbol{G}\cdot(\boldsymbol{u}(\boldsymbol{r})-\boldsymbol{u}(\boldsymbol{0}))/\rho}\right\rangle. \tag{S2}$$

Eq. (S2) is equivalent to Eq. (3) in the main text. This can be confirmed by using the microscopic definition of the displacement field

$$\boldsymbol{u}(\boldsymbol{r}) = \sum_{j=1}^{N} \boldsymbol{u}_j \delta(\boldsymbol{r}-\boldsymbol{r}_j), \tag{S3}$$

and

$$\rho_{\boldsymbol{G}}(\boldsymbol{r}) = \frac{1}{\rho}\sum_{j=1}^{N} e^{i\boldsymbol{G}\cdot\boldsymbol{u}_j}\delta(\boldsymbol{r}-\boldsymbol{r}_j). \tag{S4}$$

Since the displacement $\boldsymbol{u}(\boldsymbol{r})$ obeys a Gaussian process in the liner elastic theory in the main text, Eq. (S2) can be written as

$$\begin{aligned} C_{\boldsymbol{G}}(r) &= \exp\left[-\frac{1}{2\rho^2}\boldsymbol{G}^{\rm T}\left\langle(\boldsymbol{u}(\boldsymbol{r})-\boldsymbol{u}(\boldsymbol{0}))(\boldsymbol{u}(\boldsymbol{r})-\boldsymbol{u}(\boldsymbol{0}))^{\rm T}\right\rangle\boldsymbol{G}\right] \\ &= \exp\left[-\frac{1}{8\pi^2\rho}\int \mathrm{d}^2\boldsymbol{q}\,\left|e^{i\boldsymbol{q}\cdot\boldsymbol{r}}-1\right|^2\boldsymbol{G}^{\rm T}\mathsf{S}_{\rm u}(\boldsymbol{q})\boldsymbol{G}\right], \end{aligned} \tag{S5}$$

where the matrix elements of $\mathsf{S}_{\rm u}(\boldsymbol{q})$ are given by

$$\begin{aligned} S_{\rm u}^{(\alpha,\beta)}(\boldsymbol{q}) &= \frac{1}{\rho}\int_V \mathrm{d}^2\boldsymbol{r}\ \langle u_\alpha(\boldsymbol{r},0)u_\beta(\boldsymbol{0},0)\rangle\, e^{-i\boldsymbol{q}\cdot\boldsymbol{r}} \\ &= S_{\rm u}^{\parallel}(q)\frac{q_\alpha q_\beta}{q^2} + S_{\rm u}^{\perp}(q)\left(\delta_{\alpha,\beta}-\frac{q_\alpha q_\beta}{q^2}\right). \end{aligned} \tag{S6}$$

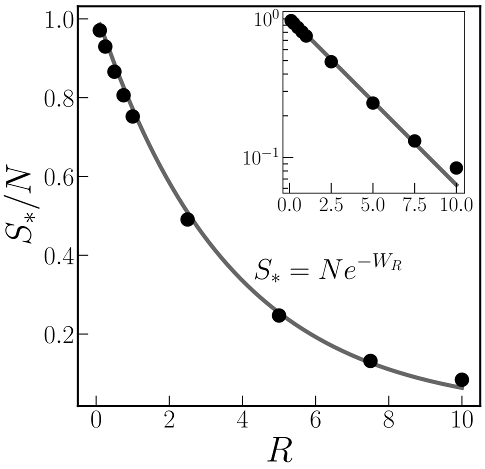


FIG. S3. The peak height of $S(\boldsymbol{q})$ at $\boldsymbol{q}=\boldsymbol{G}$, $S_* = S(\boldsymbol{G})$, as a function of $R$, at $N = 22400$. The filled circles are numerical data, and the solid line is the theoretical prediction. The inset indicates the same plot with a logarithmic scale for the vertical axis.

The second equality of Eq. (S5) follows from the relation

$$\left\langle \hat{\boldsymbol{u}}(\boldsymbol{q})\hat{\boldsymbol{u}}^{\mathrm{T}}(\boldsymbol{q}')\right\rangle = (2\pi)^2\rho \mathsf{S}_{\mathrm{u}}(\boldsymbol{q})\delta(\boldsymbol{q}+\boldsymbol{q}'). \tag{S7}$$

From Eq. (13) in the main text, we obtain

$$\begin{aligned}\boldsymbol{G}^{\mathrm{T}}\mathsf{S}_{\mathrm{u}}(\boldsymbol{q})\boldsymbol{G} &= S_{\mathrm{u}}^{\parallel}(q)\frac{(\boldsymbol{G}\cdot\boldsymbol{q})^2}{q^2} + S_{\mathrm{u}}^{\perp}(q)\left(|\boldsymbol{G}|^2 - \frac{(\boldsymbol{G}\cdot\boldsymbol{q})^2}{q^2}\right)\\ &\simeq \frac{G^2}{2}\left(S_{\mathrm{u}}^{\parallel}(q) + S_{\mathrm{u}}^{\perp}(q)\right)\\ &= \frac{G^2R^2}{4}\left[\frac{1}{1+(\xi_\parallel q)^4} + \frac{1}{1+(\xi_\perp q)^4}\right].\end{aligned} \tag{S8}$$

In the second equality, $(\boldsymbol{G}\cdot\boldsymbol{q})^2$ is replaced by the directional average value $G^2q^2/2$. Using a formula of the Bessel function of the first kind

$$J_0(z) = \frac{1}{2\pi}\int_0^{2\pi} \mathrm{d}\theta\; e^{iz\cos\theta} \tag{S9}$$

and its asymptotic behavior for large $z$, $J_0(z \gg 1) \sim z^{-1/2}\cos(z-\pi/4)$, we have

$$\begin{aligned}C_{\boldsymbol{G}}(r) &= \exp\left[-\frac{G^2R^2}{8\pi\rho}\int_0^{\Lambda_{\mathrm{c}}}\mathrm{d}q\; q(1-J_0(qr))\left\{\frac{1}{1+(\xi_\parallel q)^4} + \frac{1}{1+(\xi_\perp q)^4}\right\}\right]\\ &\sim \exp\left[-W_R + O(r^{-1/2})\right] \qquad (r\to\infty),\end{aligned} \tag{S10}$$

where

$$W_R := \frac{G^2R^2}{16\pi\rho}\left[\frac{1}{\xi_\parallel^2}\arctan\left(\Lambda_{\mathrm{c}}^2\xi_\parallel^2\right) + \frac{1}{\xi_\perp^2}\arctan\left(\Lambda_{\mathrm{c}}^2\xi_\perp^2\right)\right]. \tag{S11}$$

Thus $C_{\boldsymbol{G}}(r)$ converges to a constant in the large $r$ limit.

## S5. BRAGG PEAK

The static structure factor $S(\boldsymbol{q})$ can be written in terms of $C_{\boldsymbol{G}}(r)$ as

$$S(\boldsymbol{q}) = \rho\int_V \mathrm{d}^2\boldsymbol{r}\; e^{-i(\boldsymbol{q}-\boldsymbol{G})\cdot\boldsymbol{r}}C_{\boldsymbol{G}}(r). \tag{S12}$$

Substituting Eq. (S10) into Eq. (S12), we find that in the vicinity of the reciprocal lattice vector $\boldsymbol{G}$, $S(\boldsymbol{q})$ behaves as

$$S(\boldsymbol{q} \simeq \boldsymbol{G}) \sim N e^{-W_R} \delta_{\boldsymbol{q},\boldsymbol{G}}. \tag{S13}$$

Therefore, at $\boldsymbol{q} = \boldsymbol{G}$, $S(\boldsymbol{q})$ has a peak whose height is $N e^{-W_R}$, as we showed in Fig. 4(d) in the main text. We show $S_* = S(\boldsymbol{G})$ as a function of $R$ in Fig. S3. The filled circles represent the numerical data, and the solid line is the theoretical expression, $S_* = N e^{-W_R}$, where $W_R$ is given by Eq. (S11). We plotted the theoretical line using the numerical value of $\xi_{\parallel,\perp}$ obtained from Figs 4(a) and (b) in the main text. We set $G = 4\pi/(\sqrt{3}\ell_0)$ and the cut-off wavenumber as $\Lambda_{\mathrm{c}} = 1/\ell_0$.

## S6. RESULTS FOR FINITE PERSISTENCE TIME

In the main text, we showed the correlation functions at $D = 0$ since we are only interested in the states accompanied by hyperuniformity. Here, we show the results for the finite diffusion constant $D$ (or persistence time $\tau_{\mathrm{p}} = 1/D$).

### A. Theory

First, we derive the theoretical expressions of the displacement correlation and static structure factor. The dynamics of the coarse-grained displacement field $\boldsymbol{u}(\boldsymbol{r}, t)$ is described by

$$\partial_t \boldsymbol{u}(\boldsymbol{r}, t) = \frac{1}{\zeta} \nabla \cdot \frac{\delta \mathcal{F}[\mathsf{u}(\cdot, t)]}{\delta \mathsf{u}(\boldsymbol{r}, t)} + \boldsymbol{\Xi}(\boldsymbol{r}, t). \tag{S14}$$

The functional $\mathcal{F}[\mathsf{u}(\cdot, t)]$ is given by

$$\mathcal{F}[\mathsf{u}(\cdot, t)] = \frac{1}{2} \int_V \mathrm{d}^2\boldsymbol{r} \, \left[\lambda \mathrm{Tr}[\mathsf{u}(\boldsymbol{r}, t)]^2 + 2\mu \mathsf{u}(\boldsymbol{r}, t) : \mathsf{u}(\boldsymbol{r}, t)\right], \tag{S15}$$

where $\mathsf{u}(\boldsymbol{r}, t) = (\nabla \boldsymbol{u}(\boldsymbol{r}, t) + [\nabla \boldsymbol{u}(\boldsymbol{r}, t)]^{\mathrm{T}})/2$ is the strain tensor. $\boldsymbol{\Xi}(\boldsymbol{r}, t)$ is a Gaussian noise with zero mean and the correlation

$$\left\langle \boldsymbol{\Xi}(\boldsymbol{r}, t) \boldsymbol{\Xi}^{\mathrm{T}}(\boldsymbol{r}', t') \right\rangle = \frac{v_0^2 \rho}{2} \mathsf{R}(\Omega(t - t')) e^{-D|t-t'|} \delta(\boldsymbol{r} - \boldsymbol{r}'), \tag{S16}$$

where

$$\mathsf{R}(\theta) = \begin{pmatrix} \cos\theta & -\sin\theta \\ \sin\theta & \cos\theta \end{pmatrix}. \tag{S17}$$

The model is reduced to the equilibrium system of the effective temperature $T_{\mathrm{act}} = v_0^2 \zeta/(2D)$ in the limit $D \to \infty$ (or $\tau_{\mathrm{p}} \to 0$) because in this limit, Eq. (S16) becomes

$$\left\langle \boldsymbol{\Xi}(\boldsymbol{r}, t) \boldsymbol{\Xi}^{\mathrm{T}}(\boldsymbol{r}', t') \right\rangle = \frac{2 T_{\mathrm{act}} \rho}{\zeta} \delta(\boldsymbol{r} - \boldsymbol{r}') \delta(t - t') \mathbb{1}, \tag{S18}$$

which indicates the fluctuation-dissipation relation.

We now calculate the correlation functions in Fourier space. By decomposing the displacement field in Fourier space, $\hat{\boldsymbol{u}}(\boldsymbol{q}, \omega)$, into the longitudinal and transverse components as $\hat{\boldsymbol{u}}(\boldsymbol{q}, \omega) = \hat{u}_{\parallel}(\boldsymbol{q}, \omega) \boldsymbol{e}_{\parallel} + \hat{u}_{\perp}(\boldsymbol{q}, \omega) \boldsymbol{e}_{\perp}$, Eq. (S15) becomes

$$-i\omega \hat{u}_{\parallel}(\boldsymbol{q}, \omega) = -a_{\parallel} q^2 \hat{u}_{\parallel}(\boldsymbol{q}, \omega) + \hat{\Xi}_{\parallel}(\boldsymbol{q}, \omega), \tag{S19}$$

$$-i\omega \hat{u}_{\perp}(\boldsymbol{q}, \omega) = -a_{\perp} q^2 \hat{u}_{\perp}(\boldsymbol{q}, \omega) + \hat{\Xi}_{\perp}(\boldsymbol{q}, \omega), \tag{S20}$$

where $a_{\parallel} := (\lambda + 2\mu)/\zeta$ and $a_{\perp} := \mu/\zeta$. The dynamical correlation function is calculated as

$$S_{\mathrm{u}}^{\mathrm{X}}(\boldsymbol{q}, \omega) = \frac{1}{\omega^2 + a_{\mathrm{X}}^2 q^4} S_{\Xi}^{\mathrm{X}}(\boldsymbol{q}, \omega), \quad \mathrm{X} \in \{\parallel, \perp\}, \tag{S21}$$

where

$$
\begin{aligned}
S^{\mathrm{X}}_{\Xi}(\boldsymbol{q},\omega) &:= \frac{1}{\rho}\int_V \mathrm{d}^2\boldsymbol{r}\int_{-\infty}^{\infty}\mathrm{d}\omega\ \langle \Xi_{\mathrm{X}}(\boldsymbol{r},t)\Xi_{\mathrm{X}}(\boldsymbol{0},0)\rangle\, e^{-i(\boldsymbol{q}\cdot\boldsymbol{r}-\omega t)} \\
&= \frac{v_0^2}{2}\left[\frac{D}{D^2+(\omega+\Omega)^2}+\frac{D}{D^2+(\omega-\Omega)^2}\right].
\end{aligned}
\tag{S22}
$$

The equal time correlation function is obtained by integrating Eq. (S21) over $\omega$:

$$
S^{\mathrm{X}}_{\mathrm{u}}(\boldsymbol{q}) = \frac{1}{2\pi}\int_{-\infty}^{\infty}\mathrm{d}\omega\ S^{\mathrm{X}}_{\mathrm{u}}(\boldsymbol{q},\omega) = \frac{v_0^2}{2a_{\mathrm{X}}q^2}\frac{D+a_{\mathrm{X}}q^2}{\Omega^2+(D+a_{\mathrm{X}}q^2)^2}. \tag{S23}
$$

In the limit $D\to 0$, Eq. (S23) becomes Eq. (13) in the main text. As discussed in the main text, when $D=0$, the displacement correlations $S^{\mathrm{X}}_{\mathrm{u}}(\boldsymbol{q}\to\boldsymbol{0})$ is constant, meaning the long-range translational order. When $D>0$, however, $S^{\mathrm{X}}_{\mathrm{u}}(\boldsymbol{q})$ behaves as $S^{\mathrm{X}}_{\mathrm{u}}(\boldsymbol{q})\propto 1/q^2$ for small $q$, independent of $D$ and $\Omega$. This behavior, $S^{\mathrm{X}}_{\mathrm{u}}(\boldsymbol{q})\propto 1/q^2$, directly leads to the crystalline order being unstable.

## B. Numerical results

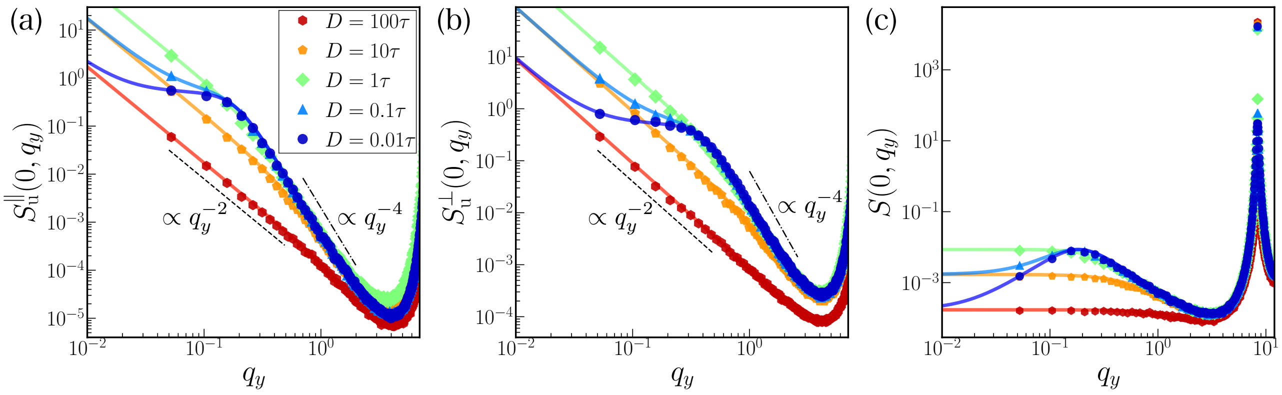


FIG. S4. The correlation functions of the longitudinal (a), transverse of the displacement (b), and the static structure factor (c) for finite rotational diffusion constant $D$ at $R=1\sigma$, $\varphi=1.209$, and $N=22400$. The solid lines represent the theoretical prediction by Eq. (S23). The fitting parameter is only $a_{\parallel,\perp}$. The fitting results are independent of $D$.

In Figs. S4 (a) and (b), we show the longitudinal and transverse displacement correlation functions in Fourier space for various $D(\neq 0)$. For large $D$, both $S^{\parallel}_{\mathrm{u}}(\boldsymbol{q})$ and $S^{\perp}_{\mathrm{u}}(\boldsymbol{q})$ behave as $1/q^2$. The behavior $1/q^2$ for large $D$ is natural because, in the limit $D\to\infty$, the cABP model [Eqs. (1) and (2) in the main text] is reduced to an equilibrium system. For small $D$, we find a plateau between the regime of $q^{-4}$ for large $q$ and $q^{-2}$ for small $q$. The plateau regime corresponds to the length scale where the translational order is long-ranged but in the thermodynamic limit, the order turns to the quasi-long-ranged due to the $q^{-2}$ regime. These results mean the long-range translational order is absent for finite $D$, even if it is very small. We also show the static structure factor in Fig. S4 (a) for various finite $D$. One observes that the hyperuniformity disappears as $D$ increases. This observation is the same as in the fluid states.
